# Supplementary material for: PolarStar: Expanding the Scalability Horizon of Diameter-3 Networks
Source: arXiv:2302.07217 source file (2024-08-06)
Supplement: Supplementary file 1 [file appendix.tex]

\section{Appendix: Supplemental Materials}\label{sec:appendix}
\subsection{Comparing the P and R Properties}\label{sec:p_r_compared}
\noindent We state the original $P$ properties introduced by Bermond et al. in \cite{bermond82}, and distinguish them from our $R$ properties. 
%We use an easily derived equivalent formulation of \ref{prop_P_star}, rather than that used in \cite{bermond82}.
\subsubsection{The P Properties}
\begin{propertyp}{P}\cite{bermond82}\label{prop_P_appendix}
A diameter-$D$ graph has Property $P$ if any pair of vertices at distance $D$ are joined by a $D+1$-hop path.
\end{propertyp}
\begin{propertyp}{P$^*$}\cite{bermond82}
\label{prop_P_star_appendix}
A graph $G$ has Property $P^*$ if it has diameter $\le 2$ and 
it is of diameter $\le 2$ and there is an involution $f$ on $G'$ such that for any $x'\in V(G)$, 
\begin{align}
V(G) &= \{x\}\cup \{f(x)\} \cup f(N(x)) \cup N(f(x)) \nonumber
\end{align}
\end{propertyp}
\if0
\begin{propertyp}{P$^*$}
\label{prop_P_star_appendix}
A graph $G$ has Property $P^*$ if it has diameter $\le 2$ and 
for any $x'$ and $y' \in G'$, at least one of the following is true: (1)~$y'=x'$, (2)~$y'=f(x')$, (3)~$(x',y') \in E(G')$, or (4)~$(f(x'),f(y')) \in E(G')$.
\end{propertyp}
\fi
%\lmedit{It is not difficult to show that Property \ref{prop_P_star} is Property \ref{prop_R_star}, but with the additional diameter $\le 2$ constraint.}
\begin{corollary}\label{cor:proppstar_eq_appendix}
    If a graph $G'$ has Property $P^*$, then for any $x'$ and $y' \in G'$, at least one of the following is true: 
(1)~$y'=x'$, (2)~$y'=f(x')$, (3)~$(x',y') \in E(G')$, or (4)~$(f(x'),f(y')) \in E(G')$.
\end{corollary}
\begin{proof}
    We choose some arbitrary $x'$ and $y'$ in $G'$. All $y'=f(z')$ for some $z' \in G'$. We assume that $1$ and $2$ do not hold for $y'$, and show that either $3$ or $4$ must be true for $y'$. 
    
    Since $1$ and $2$ do not hold for $y'$, they can not hold for $z'$. So $z' \in f(N(x')) \cup N(f(x'))$. 
        If $z' \in f(N(x'))$, $f(z') = y' \in N(x')$, and $(x',y') \in E(G')$. 
        If $z' \in N(f(x'))$, then $(f(x'),z') = (f(x'),f(y')) \in E(G')$.
\end{proof}
\begin{propertyp}{P$_i$}\cite{bermond82}\label{prop_P_i_appendix}  A graph $G'$  has Property~\ref{prop_P_i_appendix} if there is a bijection $f$, with $f^2$ an automorphism of $G'$, so that the graph $G_i$ with edges 
$
E(G') \cup f(E(G'))
$
has diameter $i$.
\end{propertyp}
%\printProofs
\subsubsection{The R Properties}
We restate the $R$ properties here for ease of reference.
\begin{propertyp}{R}
A graph $G$ of diameter $D$ has Property~\ref{prop_R} if any vertex pair $x,y\in V(G)$ 
%(not necessarily different)
can be joined by a path of length~$D$.  
\end{propertyp}
%\printProofs
\if0
\begin{lemma}\label{lemma:R_appendix}
In a graph $G$ of diameter $D$ having Property~\ref{prop_R}, there is a length $D+1$ path between any pair of vertices $x,y\in V(G)$.
\end{lemma}
\fi
\begin{propertyp}{R$^*$} A graph $G'$ 
satisfies Property~\ref{prop_R_star} if there is an involution $f$ on $G'$ so that for any $x'$ and $y' \in G'$, at least one of the following is true: 
    (1) $y'=x'$,
    (2) $y'=f(x')$,
    (3) $(x',y') \in E(G')$, or
    (4) $(f(x'),f(y')) \in E(G')$.
\end{propertyp}
\begin{corollary}
\label{cor:R_appendix}
If graph $G$ of diameter $D$ has Property~\ref{prop_R}, 
any vertex pair $x,y\in V(G)$ 
%(not necessarily different)
can be joined by a path of length~$D+1$.
\end{corollary}
\begin{proof}
    Consider any neighbor $z$ of $y$. By Property~\ref{prop_R}, there exists a path $p_D$ of length $D$ from $x$ to $z$. Appending edge $(z,y)$ to $p_D$ gives a path of length $D+1$ between $x$ and $y$.
\end{proof}
\begin{propertyp}{R$_1$}\cite{bermond82}  A graph $G'$  has Property~\ref{prop_R_1} if there is a bijection $f$, with $f^2$ an automorphism of $G'$, so that the set of edges 
$
E(G') \cup f(E(G'))
$
is the entire set of edges in the complete graph on \looseness=-1$V(G')$.
\end{propertyp}
\subsubsection{Relationship Between P and R Properties}
The $P$ and $R$ properties are related as follows:
\begin{itemize}[itemsep=0pt,parsep=2pt]
    \item R$^*$ weakens P$^*$ by allowing diameter $>2$. 
    \item R strengthens P by requiring that all vertex pairs be joined by a path of length diameter $D$. 
    \item R$_1$ is P$_1$. Note that R$_1$ (and P$_1$) imply R$^*$ if $f$ is an involution, and further imply P$^*$ if $G'$ has diameter $\le 2$. 
\end{itemize}
\begin{theorem}
    Any graph with Property R has Property P. Any graph with Property P$^*$ has Property R$^*$.
\end{theorem}
\begin{proof}
   The relationship between P and R follows from Property P and Corollary~\ref{cor:R_appendix}. The relationship between P$^*$ and  R$^*$ follows from Corollary~\ref{cor:proppstar_eq_appendix} and Property R$^*$. 
\end{proof}
Weakening Property P$^*$ permits us to design $IQ$, a $G'$ supernode graph with Property R$^*$ that may have diameter $>2$, with larger order than that feasible with property P$^*$. Use of this R$^*$-graph rather than a P$^*$-graph maintains diameter-$3$ for the star product. The structure graph, $ER_q$ from \cite{bermond82}, has both Properties P and R, so may also be used here as our structure graph.
% The $ER_q$ graph (with self-loops) has both Properties~\ref{prop_P} and \ref{prop_R}, so may be used in either construction.
%\printProofs
\subsection{Proofs of Selected Material from the Text}
\lmedit{These need to be uncommented in the text itself to see this section. They've all been incorporated into the text.}
%\printProofs
\if0
\lmedit{
\subsection{The Erd\"os-R\'enyi Polarity Graphs}
Do we really need anything here?
More discussion here, including the self-loop conversation. Maybe she the actual construction of the network.

\lmcomment{How much of this do we actually need?}
\subsubsection[Self-loops in ERq]{Self-loops in $ER_q$}
An important aspect of the ER graph is the existence of self-orthogonal vertices. There are no self-orthogonal vectors in Euclidean $3$-space but they exist in $\mathbb{F}_q^3$, giving vertices with a self-loop edge. {Self-loops are 
%essential for establishing 
used to establish Property~\ref{prop_R} in %our structure graph
$ER_q$. The possession of Property~\ref{prop_R} is sufficient for $ER_q$ to be used as a structure graph in the construction of a star product having diameter 3. %but is not always necessary, depending on the structure of $G'$.
}

Intuitively, the self-loops on ER structure graphs translate
to additional edges connecting distinct vertices within a supernode.
%, as seen in the red supernodes in Figs.~\ref{fig:star_star} and \ref{fig:star_paley}. 
There are no self-loops in PolarStar itself: we delete any self-loops that may remain in the star product, 
%as they are needed only for the proof and the construction.
as they do not affect the scale or diameter of the product graph.

{
In the supernodes corresponding to self-loop vertices of the structure graph $G$, the internal edges
%\kldelete{The edges inside the supernodes that correspond to self-loop vertices in} 
are then all edges of the original $G'$, plus the extra edges induced by the self-loops.}
%\kldelete{An example layout for $ER_3$ is shown in Figure~\ref{fig:star_er}.}
%\klcomment{The layout is not very clear in that figure.}
For extensive detail on the construction and properties of networks built on ER graphs such as \flyN, see \cite{polarfly_sc22}.
}
\fi
